# Supplementary material for: SegNeRF: 3D Part Segmentation with Neural Radiance Fields
Source: arXiv:2211.11215 source file (2022-11-22)
Supplement: Supplementary file 4 [file 4_real.tex]

\section{Varying Reconstruction Threshold}
\section{Reconstruction With vs. Without Segmentation}
\section{Real-world images}
\section{Non-zero d for 3D}
